# Supplementary material for: CoMo: A novel co-moving 3D camera system
Source: arXiv:2101.10775 ancillary file (2021-01-26)
Supplement: Supplementary file 1 [file SI.pdf]

# APPENDIX A
# EXTERNAL PARAMETERS

## A.1 Alignment with the fishing line

We set the yaw angles of the cameras by tighten a fishing line, i.e. a thin nylon line, between the two external edges of the bars, so that the fishing line crosses the gauge and it can be used as a pointer on the gauge. Denoting the long side of the L-bar with $L$ and the distance from the point where the line crosses the gauge and the side of the bar with $l$, we can measure the yaw angles as $atan(l/L)$, with the negative sign for the right camera and with the positive sign for the left camera.

At the first order approximation, which is reasonable because $\alpha_L, \alpha_R \ll 1$, the two yaw angles are equal to $l/L$. The error on this measure can then be estimated by computing the first order derivative of $\alpha_L$ and $\alpha_R$:

$$\delta\alpha_L = \frac{\delta l}{L} - \alpha_L \frac{\delta L}{L} \tag{1}$$

where $\delta l$ and $\delta L$ are the errors on the measure of $l$ and $L$ respectively.

$L$ represents the length of the bar, which is equal to 69cm (measured in the mechanical workshop with high precision instruments and then measured again in the lab with a distolaser) and the error on this measure, $\delta L$ is of the order of 1mm. Therefore $\delta L/L = 1.4 \cdot 10^{-3}$. The dominant term of the error on $\alpha_L$ is then $\delta l/L$. The error on $l$ may be estimated as the thickness of the fishing line we are using, which is of $1mm$, hence the term $\delta l/L$ is of the order of $10^{-3}$. This means that the error on $\alpha_l$ is of the order of $10^{-3}$rad as well as the error on $\alpha_R$.

## A.2 Rotational matrix

The correct computation of the rotational matrix is essential for the high accuracy of the $3D$ reconstruction. As we already stated in the main text in Section 4.4, our rotational matrix is the product of a dynamic rotational matrix that takes into account the rotation of the camera due to the stage, and a static rotational matrix that takes into account the orientation of the cameras in the *home* configuration.

We start here from the computation of the static rotation matrix, which in the main text we defined as:

$$R_S(\alpha_c, \beta_c, \gamma_c) = R_{z_C}(-\gamma_c) R_{x_C}(-\beta_c) R_{y_C}(-\alpha_c) \tag{2}$$

where $x_c$, $y_c$ and $z_c$ are the three axis of the camera reference frame defined in Section 4.1 of the manuscript and $\alpha_c$, $\beta_c$ and $\gamma_c$ are the yaw, pitch and roll angles respectively.

To obtain eq.(2) we need to describe in detail the alignment procedure, the camera set-up procedure and the hardware mechanism of the head of the tripod.

Each camera is mounted on a rotational stage that is locked on a L-shape bar, see Fig.2 of the manuscript. Each bar is mounted on a tripod Manfrotto 475B with the Studio Geared Head Manfrotto 400. We set-up the yaw, pitch and roll angles of the cameras by rotating the knobs of the head of the tripod. The L-bars have a gauge on their small edge (on the left side for the right camera and on the right side for the left camera), see Fig.2 of the manuscript. During the alignment procedure we first tighten a fishing line between the two external edges of the bars, so that the line crosses the gauges, and then we set the yaw angle by rotating the bars until the line crosses the gauges at a specific mark.

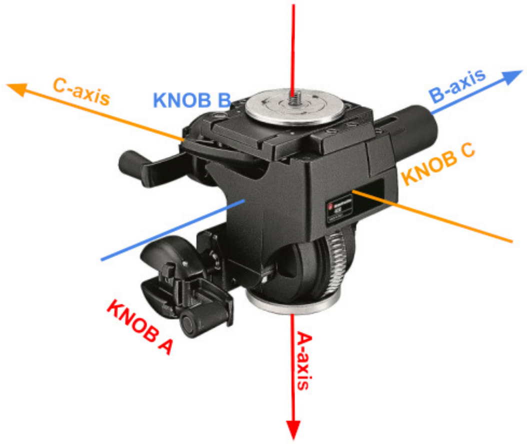


Fig. 1. **Tripod.** We use a Gear Head Manfrotto 400. The knob A controls the yaw angle rotating about the A-axis, highlighted in red. The knob B controls the pitch angle rotating around the B-axis, highlighted in blue. The knob C controls the roll angle rotating about the C-axis, highlighted in orange.

The cameras set-up procedure is the following:

**Step 1:** level the tripod;
**Step 2:** set the roll angle, $\gamma$, of both cameras to 0rad rotating knob $C$, see Fig.1;
**Step 3:** set the pitch angle, $\beta$, of both cameras to 0rad rotating knob $B$;
**Step 4:** set the yaw angles rotating the knob A to 0rad for both cameras, with the alignment procedure described above.
**Step 5:** set the yaw angles rotating the knob A to $0.11$rad for the left camera, $\alpha_L$, and to $-0.11$rad for the right camera, $\alpha_R$, with the alignment procedure described above.
**Step 6:** set the pitch angle of both cameras to $0.22$rad, rotating knob $B$.

The crucial point of the set-up procedure is to understand if and how a rotation of one of the three knobs of the tripod may affect the position of the others. Each knob is associated to a rotational axis, in this way defining a tripod reference frame with axes $A$, $B$ and $C$, which correspond to the $x_c$, $y_c$ and $z_c$ axes of the camera reference frame respectively. The relevant property of the three rotations about the tripod axes is that they are not independent from each other, see Fig.2, and in particular:

**1- Rotation of knob A.** It changes the position of knob B and knob C and therefore it changes the orientation of the B-axis and of the C-axis;
**2- Rotation of knob B.** It changes the position of knob C and therefore it changes the orientation of the C-axis, but it keeps the A-axis fixed;
**3- Rotation of knob C.** It keeps both the A-axis and the B-axis fixed.

In the set-up procedure, from step 1 to step 4 we are aligning the tripod reference frame to the world reference frame. In step 1, where we level the tripod, we are setting the $A$-axis parallel to the direction of the gravity, hence

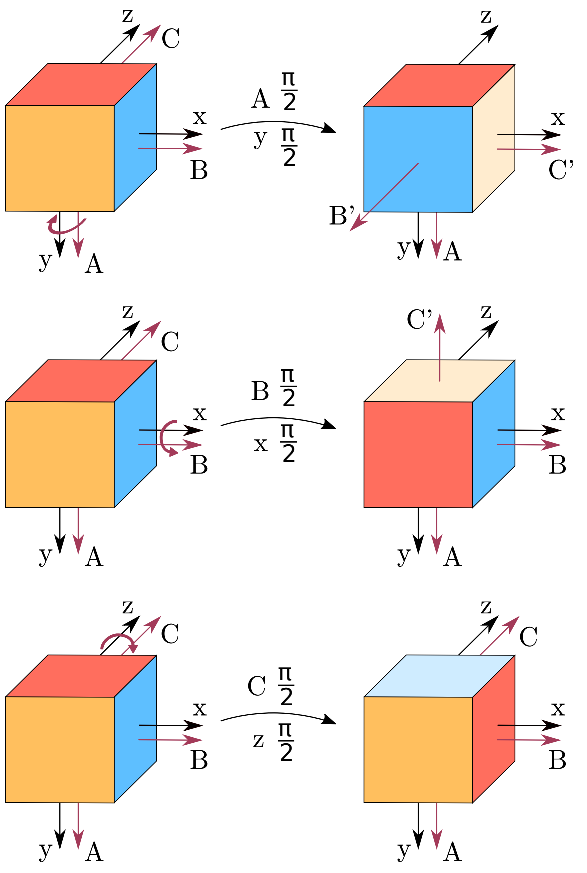


Fig. 2. **Tripod axis order.** The rotation about the 3 axis of the tripod head are not independent. We represent the tripod as a cube. Opposite faces are represented with the same color but with different intensity: dark and light red, dark and light blue, dark and light orange. For the sake of simplicity we consider all rotations of $\pi/2$rad. **First row.** A rotation about the A-axis keeps the red face fixed while rotating the blue and the orange faces. The $B$-axis is moved into $B'$ and the $C$-axis into $C'$. **Second row.** A rotation about the $B$-axis keeps the blue face fixed while rotating the red and the orange faces. The $A$-axis is not affected by the rotation, while the $C$-axis is moved into $C'$. **Third row.** A rotation about the $C$-axis keeps the orange face fixed, while rotating the red and the blue faces. Both $A$-axis and $B$-axis are not affected by the rotation.

parallel to the $y$-axis of the world reference frame. In step 2 and step 3, where we set the roll and pitch angles at 0rad, we are setting the $BC$-plane of the tripod reference frame parallel to the $xz$-plane of the world reference frame. Finally in step 4, where we set the yaw angle to 0rad we are setting the $B$-axis parallel to the direction of the vector $O_LO_R$ that connects the centers of the two cameras, which is by definition the direction of the $x$-axis in the world reference frame and for the right hand rule we will have also $C$-axis of the tripod reference frame parallel to the $z$-axis of the world reference frame.

Step 5 and step 6 of the set-up procedure are then the only relevant steps for the computation of the rotation matrix, $R$, that brings the world reference frame into the tripod reference frame. In step 5 we rotate about the $A$-axis of an angle $\alpha$. This rotation moves the $B$-axis into $B'$, about which we will rotate in step 6 of an angle $\beta$. $R$ is then of the following form:

$$R = R_{B'}(\beta)R_A(\alpha) \tag{3}$$

and noting that:

$$R_{B'} = R_A(\alpha) \cdot R_B(\beta) \cdot R_A(-\alpha) \tag{4}$$

we have that:

$$R = R_A(\alpha) \cdot R_B(\beta) \tag{5}$$

which can be expresses in terms of rotations about the axes of the world reference frame as:

$$R = R_y(\alpha) \cdot R_x(\beta) \tag{6}$$

Note that we would have obtained eq.(5) also performing the rotations in step 5 and step 6 in the reverse order, because the rotation about the $B$-axis does not change the orientation of the $A$-axis. Therefore regardless the order of the rotations performed at step 5 and step 6, the rotation matrix is of the form in eq.(5).

In a more general case, where also the knob $C$ is involved in the initial set-up the combination of the three rotations is even more interesting. The non-independence of the tripod rotation axis makes the order of rotation not relevant anymore. Indeed, regardless the order of the composition, a rotation of an angle $\alpha$ around the $A$-axis, a rotation of an angle $\beta$ around the B-axis and a rotation of an angle $\gamma$ around the C-axis, give the same resulting matrix, $R$, that can be written as, see Fig.3:

$$R = R_y(\alpha)R_x(\beta)R_z(\gamma) \tag{7}$$

Note that eq.(7) is trivially verified when we first rotate of an angle $\gamma$ about the $C$-axis, then we rotate of an angle $\beta$ about the B-axis and finally of an angle $\alpha$ about the A-axis, see the first row of Fig.3.

We make here the explicit computation for the worst case scenario, when we first apply a rotation of $\alpha$ about the A-axis, then a rotation of $\beta$ about the $B$-axis and finally a rotation of $\gamma$ around $C$-axis, see the second row of Fig.3. The first rotation of $\alpha$ moves $B$ to $B'$ and $C$ to $C'$. $C'$ is again moved to $C''$ by the rotation of $\beta$ and our final rotation is given by $R = R_{C''}(\gamma)R_{B'}(\beta)R_A(\alpha)$. $R_{B'}(\beta)$ verifies eq.(4), while for $R_{C''}$ the following equation holds:

$$\begin{aligned} R_{C''} = \; & R_{B'}(\beta)R_{C'}(\gamma)R_{B'}(-\beta) = \\ = \; & R_{B'}(\beta)R_A(\alpha)R_C(\gamma)R_A(-\alpha)R_{B'}(-\beta) = \\ = \; & R_A(\alpha)R_B(\beta)R_C(\gamma)R_B(-\beta)R_A(-\alpha) = \\ = \; & R_y(\alpha)R_x(\beta)R_z(\gamma)R_x(-\beta)R_y(-\alpha) \end{aligned} \tag{8}$$

Therefore:

$$\begin{aligned} R = \; & R_{C''}(\gamma)R_{B'}(\beta)R_A(\alpha) \\ = \; & R_y(\alpha)R_x(\beta)R_z(\gamma) \end{aligned} \tag{9}$$

We obtain exactly the same result with all the permutations of the rotations about the 3 axes. We show in Fig.3 three of the six permutations of the rotations. For the sake of simplicity in the visualization of the rotations in Fig.3 we consider the case where all the angles of rotation are equal to $\pi/2$.

The matrix $R$ defines the rotation that brings the world reference frame into the camera reference frame, but we need its inverse:

$$R^{-1} = R_z(-\gamma)R_x(-\beta)R_y(-\alpha) \tag{10}$$

and we need to express this rotation in the camera reference frame, i.e. we need to define $R^{-1}$ as a combination of rotations about the axis $x_c$, $y_c$ and $z_c$.

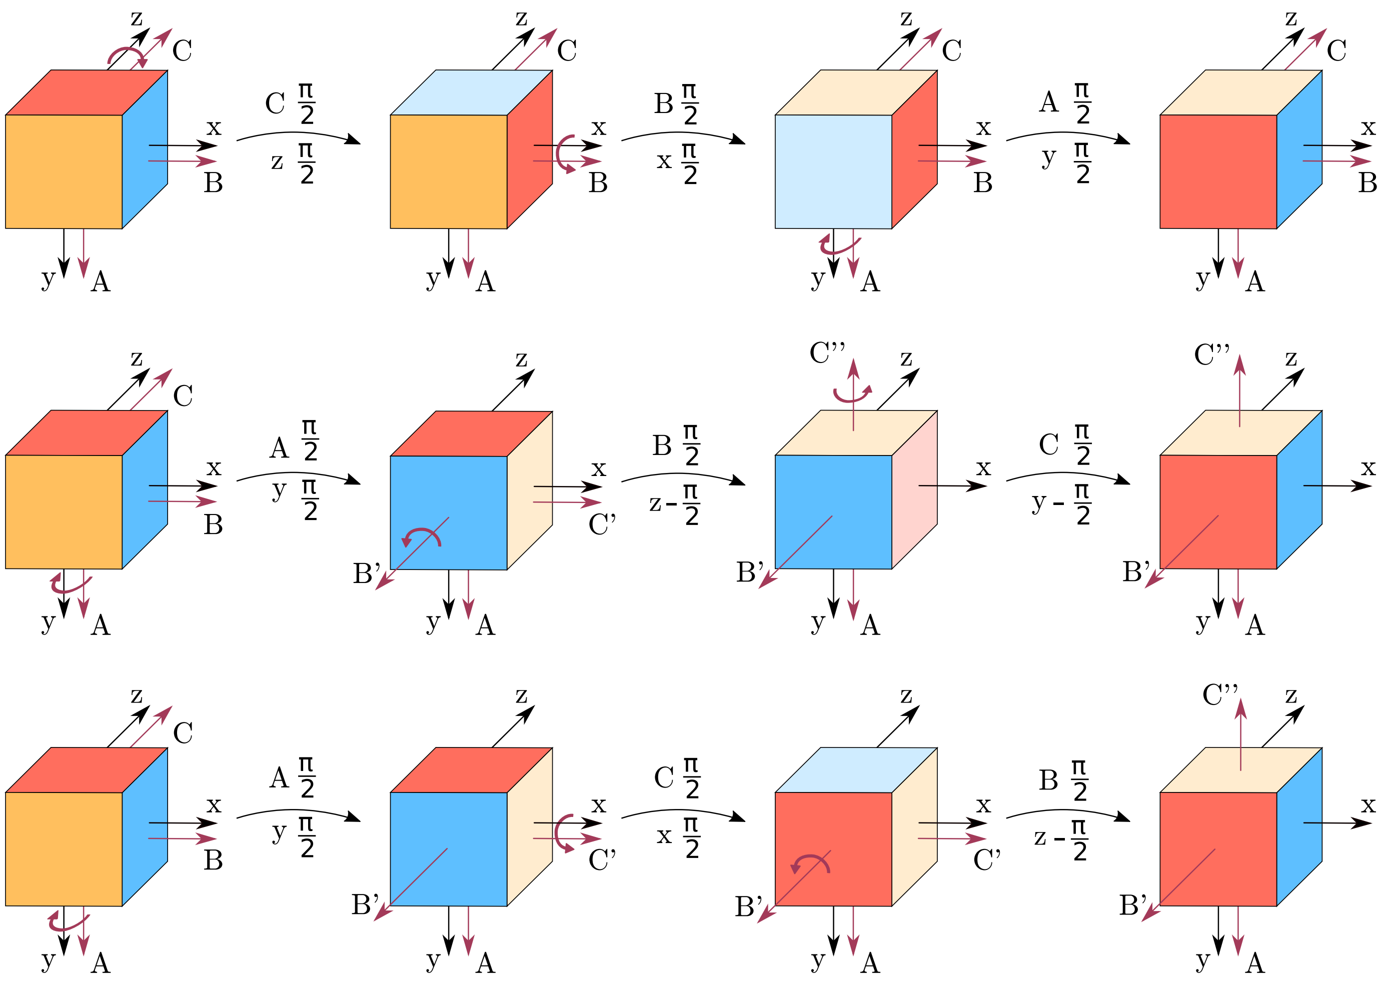


Fig. 3. **Rotations order.** We represent the tripod as a cube. Opposite faces are represented with the same color but with different intensity: dark and light red, dark and light blue, dark and light orange. For the sake of simplicity we consider all rotations of $\pi/2$rad. A rotation of an angle $\alpha$ about the $A$-axis, of an angle $\beta$ about the $B$-axis and a rotation of an angle $\gamma$ about the $C$-axis produce the same final position of the tripod regardless the order with which the rotations are performed: starting from the same position (first column) and performing the rotations in different order (different rows) the tripod final position is always the same (fourth column). **First row.** Performing first a rotation about the C-axis, then about the B-axis and finally about the A-axis, the three axis of rotations do not change their directions and we end up with the cube with the red face in front, the blue face on the right and the light orange face on top. **Second row.** Performing first a rotation about the A-axis, then about the B-axis and finally about the C-axis, we end up with the cube with the red face in front, the blue face on the right and the light orange face on top as in the first row, but the $B$-axis moved to $B'$ pointing inward and the $C$-axis moved to $C''$ pointing up. **Third row.** Performing first a rotation about the A-axis, then about the C-axis and finally about the B-axis, we end up with the cube with the red face in front, the blue face on the right and the light orange face on top as in the first two rows, but the $B$-axis moved to $B'$ pointing inward and the $C$-axis moved to $C''$ pointing up.

The following equations define the correspondence between the rotations about the axes of the camera reference frame and the rotations about the world reference frame:

$$\begin{cases} R_{x_C}(\beta) = & R\cdot R_x(\beta)\cdot R^{-1} \\ R_{y_C}(\alpha) = & R\cdot R_y(\alpha)\cdot R^{-1} \\ R_{z_C}(\gamma) = & R\cdot R_x(\gamma)\cdot R^{-1} \end{cases} \tag{11}$$

Therefore the product of the three matrices $R_{y_C}(-\alpha)$, $R_{x_C}(-\beta)$ and $R_{z_C}(-\gamma)$ is equal to $R^{-1}$ and hence:

$$R_S = R_{z_C}(-\gamma)R_{x_C}(-\beta)R_{y_C}(-\alpha) \tag{12}$$

Therefore the camera rotational matrix, $R_S$ is of the form defined at the beginning of this section in eq.(2).

To compute the full rotational matrix we need to compose $R_S$ with the dynamic rotation matrix due to the stage, which is already defined in the camera reference frame as a rotation of $\varphi(t)$ around the $y_c$-axis. Therefore the full rotation matrix is:

$$R_C(t) = R_{y_C}(\varphi(t))R_{z_C}(-\gamma)R_{x_C}(-\beta)R_{y_C}(-\alpha) \tag{13}$$

## Appendix B
## Motion device

The motion device for the online motion mode consists of a Raspberry Pi 3 Model B+ with the Pi Touchscreen 7″ and a joypad Logitech F310, as in the scheme of Fig.4. The Raspberry Pi is used on one side to redirect to the unit control the input signals received from the joypad and from the touch screen, on the other side to read and store the data gathered from the unit controller.

The user chooses the rotational velocity, which is then sent to the Raspberry Pi and hence to the unit controller,

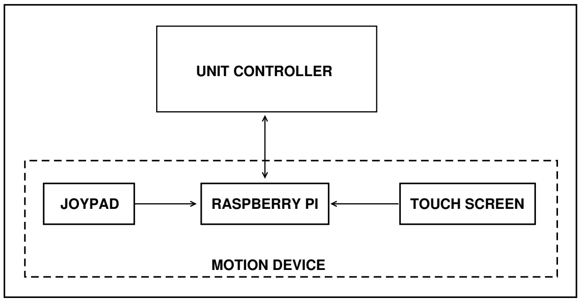


Fig. 4. **Motion Device.** The motion device consists of a Raspberry Pi 3 Model B+ with Pi Touchscreen $7''$ and a joypad Logitech F310. The Raspberry Pi is used on one side to redirect to the unit control the input signals received from the joypad and the touch screen, on the other side to read and store the data gathered from the unit controller. The user chooses the rotational velocity moving the stick of the joypad, while the touchscreen is used to display the control program interface.

by moving the stick of the joypad. The relationship between the joystick position and rotational velocity is given by

$$V = \begin{cases} xV_{max} & \text{for } |x| > 0.2 \\ 0 & \text{for } |x| \leq 0.2 \end{cases} \quad (14)$$

where $V$ is the rotational velocity, $V_{max}$ is the maximum rotation speed previously set in the unit controller, $x \in [-1, 1]$ is the range of the user input value, i.e. $x = 1$ corresponds to the user pushing the stick to the right at the joystick end of stroke while $x = -1$ corresponds to the user pushing the stick to the left at the joystick end of stroke. The direction of the rotation is set by the direction of the stick: when the stick is pushed to the right, $x > 0$, the stages will rotate in clockwise direction while when the stick is pushed to the left, $x < 0$, the stages will rotate in counterclockwise direction. Finally, for $x$ in the range between $-0.2$ and $0.2$ the rotational velocity is set to $0$ to cut down and accidental movement cause by *jitter*.

The touchscreen is used to display the control program interface, see Fig.5, which may be divided into three parts:
**1. System status indicator.** It gives information on the current status of the system.
**2. Stages position display.** It gives the information on the position of the stages.
**3. Function buttons.** It includes four buttons that the user may push to activate the correspondent functionality. The START button is used to check the working status of each part of the system. If this button is activated, the program will check whether the joystick is connected properly and establish a TCP connection with the unit controller. The HOME button is used to restore the stage to the *home* position, i.e. rotation of $0°$. The ARM button is used to engaged/disengaged the stages. When this button is activated, the control program will continuously detect the joystick position information and convert it into a velocity control command to send to the unit controller. The REC button is used to control the stage position recording function of the unit controller. When the button is activated, the internal timer and buffer of the unit controller are on standby and waiting for the trigger signal to start gathering the stages position.

The workflow of the motion device is the following: 1. Turn on the power supply of the unit controller and the

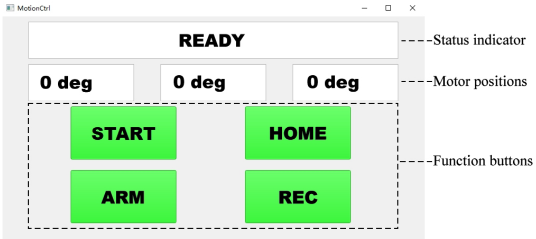


Fig. 5. **Interface.** The interface may be divided into $3$ parts: **1. System status indicator** that gives information on the current status of the system; **2. Stages position display** that show online the position of the three stages; **3. Function buttons** that includes four buttons that the user may activate. The START button is used to check the working status of each part of the system. If this button is activated, the program will check whether the joystick is connected properly and establish a TCP connection with the unit controller. The HOME button is used to restore the stage to the *home* position, i.e. rotation of $0°$. The ARM button is used to engaged/disengaged the stages. When this button is activated, the control program will continuously detect the joystick position information and convert it into a velocity control command to send to the unit controller. The REC button is used to control the stage position recording function of the unit controller. When the button is activated, the internal timer and buffer of the unit controller are on standby and waiting for the trigger signal to start gathering the stages position.

Raspberry Pi; 2. Use the Raspberry Pi to perform a self-check to confirm that the system components are ready for operation; 3. Activate the HOME button; 4. Activate the ARM button; 5. Activate the REC button; 6. At the end of the data acquisition, the Raspberry Pi reads the stages position gathered by the unit controller buffer and save it.

## Appendix C
## Stage home repeatability evaluation

In the rotational stage *home* procedure performed at the end of each acquisition, we include the initialization of the stage, namely we first initialize the stage and then we move the stage to the home position. The unit controller offers also a direct procedure to home the stage from a generic position, but we chose the indirect procedure because of its higher consistency in terms of repeatability of the home position.

We cannot have an absolute measure of the home position, hence we estimated the home position fluctuations. We performed a series of tests to evaluate the fluctuations in different conditions. Each test consists of a set of $100$ images of seven targets ($2 \times 2$ checkerboard) collected with the camera mounted on the stage, and with the stage sent to the home position after performing an action, which may be the initialization of the stage followed by the homing procedure or a controlled rotation of the stage followed by the homing procedure. We detect the targets on the images with the subpixel routine [1] that associates to each target the position of its central corner, and we measure the angular fluctuation of the home position within each pair of consecutive images as the displacement of the targets, normalized by the camera focal length $\Omega$.

For each test, we compute the probability distribution functions (PDF) of the home position fluctuations, see Fig.6. Note that with these fluctuations measure the variability of the home positions within two consecutive images, i.e. acquisition-to-acquisition fluctuations, and not the *absolute*

variability with respect to the *correct* home positions, which we cannot measure. We need to be careful in the interpretation of these results. The acquisition-to-acquisition fluctuation is a cumulative quantity, i.e. if we have a fluctuation $f_1$ between the first and the second acquisitions and a fluctuation $f_2$ between the second and the third acquisition, we will have a fluctuation $f_1 + f_2$ between the first and the third acquisitions.

The cumulative characteristics of the fluctuations implies that there are two crucial factors in the interpretation of the PDF that we need to take care of: i. the range of the fluctuations, which gives a measure of the variability of the home position ii. the median value of the fluctuations, which gives the measure of the typical difference between two consecutive acquisitions. If the PDF of the fluctuations has a non-zero median value, i.e. $m > 0$, we may expect that if we repeat the measure $N$ times we find that the difference between the first and the last measure is $N \cdot m$, which is still positive and grows with $N$: the highest $N$ the highest the difference in the home position between the first and the last measure. On the opposite, if the median value is $0$, we may expect that repeating the measure $N$ times we find the difference between the first and the $N$-th measure close to $0$. Our choice of the indirect homing procedure against the direct one is essentially motivated to the median values of the fluctuation distribution, which is zero in the indirect procedure while it is non-zero (with a sign that depends on the direction of the rotation performed by the stage) in the direct procedure, as shown in Fig.6

More in detail, we performed the following tests.

**Test0: Reference.** We acquired a set of 100 images with the stage still in the home position, to evaluate the natural fluctuations in the targets detection routine due to the noise on the images. We found a PDF, highlighted in black in Fig.6, with a zero median and with fluctuations smaller than $6.2 \cdot 10^{-5}$rad. This distribution is used as a reference for all the other tests, because it gives the measure of the resolution of the method we are using.

**Test1: Initialization.** We acquired a set of 100 images with the stage in the home position, after performing the initialization and homing procedures. The PDF is shown in Fig.6a, where it is highlighted in purple. The plot shows the high compatibility of this PDF with the reference one, with a median value of $4.7 \cdot 10^{-7}$rad and a maximum fluctuation smaller than $4.6 \cdot 10^{-6}$rad.

**Test2: Unidirectional rotation.** We tested the home repeatibility after a rotation of the stage in one direction. To this aim we acquired six sets of images. In the first three sets, each of 100 images, we acquired the data with the stage in the home position after a clockwise rotation, i.e. positive rotation, of an angle $\varphi$ equal to $10\,\mathrm{deg}$, $25\,\mathrm{deg}$ and $45\,\mathrm{deg}$ respectively in the three tests. In the last three sets, each of 100 images, we acquired the data with the stage in the home position after a counterclockwise rotation, i.e. negative rotation, of an angle $\varphi$ equal to $-10\,\mathrm{deg}$, $-25\,\mathrm{deg}$ and $-45\,\mathrm{deg}$ respectively in the three tests. We did not find any particular trend with the angle $\varphi$, hence in Fig.6b we show the overall PDF of the fluctuations of the three tests with the positive rotation, highlighted in purple, and the overall PDF of the fluctuations of the three tests with the negative rotation, highlighted in green. Both the PDFs are compatible with the

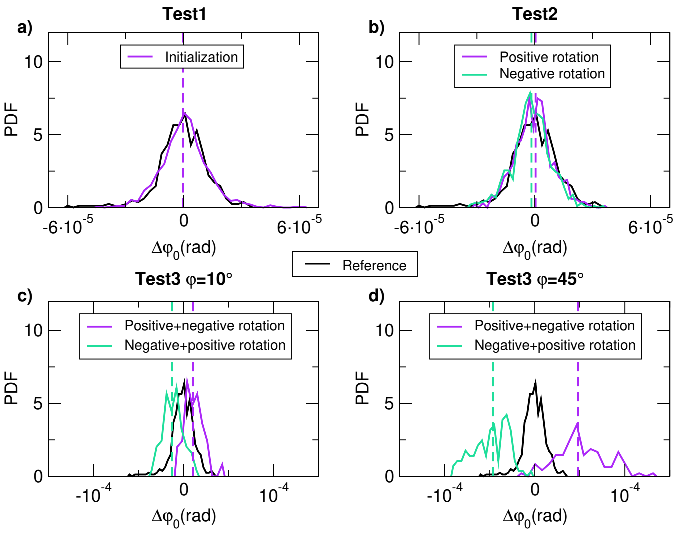


Fig. 6. **Home repeatibility.** The probability distribution function (PDF) obtained while acquiring images with the stage still represents the reference distribution for all the tests, highlighted in black in all the panels. The reference distribution gives the measure of the fluctuations due to the targets detection routine. **a) Test1.** The PDF of the fluctuations on the home position of the stage, highlighted in purple, obtained homing the stage after its initialization procedure. The PDF is compatible with the reference distribution, with the fluctuations smaller than $4.6 \cdot 10^{-5}$rad and with the median value, highlighted with the purple dashed line, equal to $4.6 \cdot 10^{-7}$rad. **b) Test2.** The PDFs of the fluctuations on the home position, after a unidirectional rotation of the stage in the positive direction, highlighted in purple, and in the negative direction, highlighted in green. Both the PDFs are compatible with the reference distribution, with the fluctuations due to the positive and negative rotations smaller than $5.7 \cdot 10^{-5}$rad and $6.1 \cdot 10^{-5}$rad respectively and with the median values equal to $-4.7 \cdot 10^{-7}$rad for the positive rotations, highlighted with the purple dashed line, and to $-1.7 \cdot 10^{-6}$rad for the negative rotations, highlighted with the green dashed line. **c) and d) Test3.** The PDFs of the fluctuations on the home position, after bidirectional rotation of the stage, namely the stage is rotated of an angle $\varphi$ in one direction and then brought to the position corresponding to $-\varphi$ with a rotation in the opposite direction. The PDFs of the tests where the first rotation is in the positive directions are highlighted in purple, the ones starting with a negative rotation are highlighted in green. The dashed lines represent the median values of the correspondent PDF. The PDFs present a trend with $\varphi$: the highest the angle $\varphi$ the further the PDFs median values from the $0$ and the higher the fluctuations. This trend is shown in panel c), where we present the results of the test with $\varphi = 10\,\mathrm{deg}$, and in panel d), where we present the results of the test with $\varphi = 45\,\mathrm{deg}$.

reference one, although we find a slightly negative median equal to $-1.7 \cdot 10^{-6}$rad for the tests with the positive rotation and a slightly positive median equal to $4.7 \cdot 10^{-7}$rad for the tests with the negative rotation.

**Test3: Bidirectional rotation.** We tested the home repeatibility after a rotation of the stage in two directions. To this aim we acquired six sets of images. In the first three sets, each of 100 images, we acquired the data with the stage in the home position after a first positive rotation of an angle $\varphi$ and then a second negative rotation from $\varphi$ to $-\varphi$. In the first three sets, each of 100 images, we acquired the data with the stage in the home position after a first negative rotation of an angle $\varphi$ and then a second positive rotation from $-\varphi$ to $\varphi$. In both cases we tested three different values of $\varphi$ equal to $10\,\mathrm{deg}$, $25\,\mathrm{deg}$ and $45\,\mathrm{deg}$. The set-up of this test is the most similar to our field set-up, where we start with the stage in the home position, we rotate in one direction to catch the flock and we rotate in the other direction while

chasing it. The PDFs for this test show the median value of the fluctuations that depends on the angle $\varphi$: the higher $\varphi$ the further the median from 0. In Fig.6c and Fig.6d we show the two cases with $\varphi$ equal to $10\,\text{deg}$ and $45\,\text{deg}$ respectively.

In all the tests we found fluctuations much smaller than the nominal one equal to $3 \cdot 10^{-4}$rad guaranteed by the factory. The comparison within the different tests show that the most accurate procedure is the one including the initialization of the stage before the homing procedure, which is the one we adopted in the design of CoMo.

## APPENDIX D
## THE SPECIAL CONFIGURATION WITH PITCH AND ROLL ANGLES EQUAL TO 0

In the special situation where the pitch and roll angles of the cameras are set to 0 we can explicitly write the solution, $\mathbf{Q}$, of the $3D$ reconstruction system:

$$\begin{cases} \mathbf{q}_L = & P_L(t) \cdot \mathbf{Q} \\ \mathbf{q}_R = & P_R(t) \cdot \mathbf{Q} \end{cases} \tag{15}$$

where $\mathbf{q}_L$ and $\mathbf{q}_R$ are the $2D$ projective points corresponding to the two images, on the left and on the right camera, $q_L$ and $q_R$ and $\mathbf{Q} = (X, Y, Z, 1)$ is the $3D$ homogeneous projective point corresponding to the $3D$ point $Q$. $P_L(t) = KR_L(t)[I| - C_L]$ and $P_R(t) = KR_R(t)[I| - C_R]$, where $R_L(t)$ and $R_R(t)$ are the two rotational matrices defined as in eq.(13), and $C_L$ and $C_R$ are two vectors of the camera centers, i.e. $C_L = (-d/2, 0, 0)$ and $C_R = (d/2, 0, 0)$.

For the sake of simplicity, in the equation above we assume that the two cameras have the same focal length, $\Omega$, and we express the position of the images $q_L$ and $q_R$ in the $2D$ reference frame with the origin on the image center, hence $K_L = K_R$ and they can be both expressed as $K$:

$$K = \begin{pmatrix} \Omega & 0 & 0 \\ 0 & \Omega & 0 \\ 0 & 0 & 1 \end{pmatrix} \tag{16}$$

Since pitch angles, $\beta_L$ and $\beta_R$, and roll angles, $\gamma_L$ and $\gamma_R$, are equal to 0 the two rotational matrices are of the form:

$$R_L(t) = R_{y_L}(-\psi_L(t)) \tag{17}$$

and

$$R_R(t) = R_{y_R}(-\psi_R(t)) \tag{18}$$

with $\psi_L(t) = \alpha_L + \varphi_L(t)$ and $\psi_R(t) = \alpha_R + \varphi_R(t)$.

The explicit form of the two matrices is then:

$$R_L = \begin{pmatrix} \cos(\psi_L(t)) & 0 & -\sin(\psi_L(t)) \\ 0 & 1 & 0 \\ \sin(\psi_L(t)) & 0 & \cos(\psi_L(t)) \end{pmatrix} \tag{19}$$

$$R_R = \begin{pmatrix} \cos(\psi_R(t)) & 0 & -\sin(\psi_R(t)) \\ 0 & 1 & 0 \\ \sin(\psi_R(t)) & 0 & \cos(\psi_R(t)) \end{pmatrix} \tag{20}$$

and in the first order approximation for $\psi_L(t), \psi_R(t) \ll 1$ we can write the last two equations as:

$$R_L = \begin{pmatrix} 1 & 0 & -\psi_L(t) \\ 0 & 1 & 0 \\ \psi_L(t) & 0 & 1 \end{pmatrix} R_R = \begin{pmatrix} 1 & 0 & -\psi_R(t) \\ 0 & 1 & 0 \\ \psi_R(t) & 0 & 1 \end{pmatrix} \tag{21}$$

Therefore the two projective matrices are of defined as:

$$P_L = \begin{pmatrix} \Omega & 0 & -\Omega\psi_L(t) & \Omega d/2 \\ 0 & \Omega & 0 & 0 \\ \psi_L(t)) & 0 & 1 & \psi_L(t)d/2 \end{pmatrix} \tag{22}$$

and

$$P_R = \begin{pmatrix} \Omega & 0 & -\Omega\psi_R(t) & -\Omega d/2 \\ 0 & \Omega & 0 & 0 \\ \psi_R(t) & 0 & 1 & \psi_R(t)d/2 \end{pmatrix} \tag{23}$$

The equation $\mathbf{q_L}^T = P_L\mathbf{Q}^T$ can then be explicitly write as:

$$\begin{cases} \bar{u}_L = & \Omega X - \Omega\psi_L(t) + \Omega d/2 \\ \bar{v}_L = & \Omega Y \\ \bar{w}_L = & \psi_L(t)X + Z + \psi_L(t)d/2 \end{cases} \tag{24}$$

and in the further approximation that $Z \gg X\psi_L(t)$ and $Z \gg \psi_L(t)d/2$ we have that:

$$\begin{cases} u_L = & \dfrac{\Omega X}{Z} - \Omega\psi_L(t) + \dfrac{\Omega d}{2Z} \\ \\ v_L = & \dfrac{\Omega Y}{Z} \end{cases} \tag{25}$$

with a similar argument we find that:

$$\begin{cases} u_R = & \dfrac{\Omega X}{Z} - \Omega\psi_R(t) - \dfrac{\Omega d}{2Z} \\ \\ v_R = & \dfrac{\Omega Y}{Z} \end{cases} \tag{26}$$

From eq.(25) and eq.(26) we obtain:

$$u_L - u_R = \Omega\psi(t) + \frac{\Omega d}{Z} \tag{27}$$

where $\psi(t) = \psi_R(t) - \psi_L(t)$, hence:

$$Z = \frac{\Omega d}{s(t) - \Omega\psi(t)} \tag{28}$$

where $s(t) = u_L(t) - u_R(t)$.

Eq.(28) gives the explicit expression for $Z$ that we already wrote as eq.(7) in the manuscript.

From the 2 system (25) and system (26) we can also compute $X$ and $Y$. In particular:

$$u_L + u_R = 2\frac{\Omega X}{Z} - \Omega(\psi_L(t) + \psi_R(t)) \tag{29}$$

and

$$v_L + v_R = 2\frac{\Omega Y}{Z} \tag{30}$$

which give:

$$\begin{cases} X = & Z\left[\dfrac{\bar{u}}{\Omega} + \bar{\psi}(t)\right] \\ \\ Y = & Z\dfrac{\bar{v}}{\Omega} \end{cases} \tag{31}$$

where $\bar{u} = (u_L + u_R)/2$, $\bar{v} = (v_L + v_R)/2$ and $\bar{\psi} = (\psi_L + \psi_R)/2$. The equations above clearly show the dependence on both $X$ and $Y$ from $Z$, and noting also that $u, v \ll \Omega$ we have that $|Q| \equiv Z$.

We obtain an explicit expression for the reconstruction error on $Z$ by deriving eq.(28):

$$\begin{aligned}\delta Z = \quad & \frac{d}{s-\Omega\psi}\delta\Omega + \frac{\Omega}{s-\Omega\psi}\delta d + \\ - \quad & \frac{\Omega d}{(s-\Omega\psi)}\left[\delta s - \delta\psi\Omega - \delta\Omega\psi\right]\end{aligned} \tag{32}$$

Substituting eq.(28) in eq.(32) we obtain:

$$\delta Z = Z\left[\frac{\delta\Omega}{\Omega} + \frac{\delta d}{d}\right] + \frac{Z^2}{\Omega d}\left[-\delta s + \delta\psi\Omega + \delta\Omega\psi\right] \tag{33}$$

Note that in the $3D$ test we use $2 \times 2$ checkerboards as targets, and we detect their position via the subpixel routine described in [1] implemented with OpenCV. Therefore for all practical purposes the error on $s$ in negligible and we can consider the following expression for $\delta Z$:

$$\delta Z = Z\left[\frac{\delta\Omega}{\Omega} + \frac{\delta d}{d}\right] + \frac{Z^2}{\Omega d}\left[\delta\psi\Omega + \delta\Omega\psi\right] \tag{34}$$

and the relative error on $Z$ is then:

$$\frac{\delta Z}{Z} = \left[\frac{\delta\Omega}{\Omega} + \frac{\delta d}{d}\right] + \frac{Z}{\Omega d}\left[\delta\psi\Omega + \delta\Omega\psi\right] \tag{35}$$

which is eq.(8) of the manuscript.

Now consider, as in the $3D$ tests, two targets, $Q_1 = (X_1, Y_1, Z_1)$ and $Q_2 = (X_2, Y_2, Z_2)$, and define $\Delta Z = Z_1 - Z_2$. The error on $\Delta Z$, $\delta(\Delta Z)$ is the difference between the error on $Z_1$ and the error on $Z_2$: $\delta(\Delta Z) = \delta Z_1 - \delta Z_2$. From eq.(32) it is then:

$$\delta(\Delta Z) = \Delta Z\left[\frac{\delta\Omega}{\Omega} + \frac{\delta d}{d}\right] + \Delta Z\frac{2\bar{Z}}{\Omega d}\left[\delta\psi\Omega + \delta\Omega\psi\right] \tag{36}$$

where $\bar{Z}$ is the average between $Z_1$ and $Z_2$, $\bar{Z} = (Z_1+Z_2)/2$ and where we have used the equation $Z_1^2 - Z_2^2 = (Z_1 - Z_2)(Z_1 + Z_2)$.

The relative error on $\Delta Z$ is then:

$$\frac{\delta(\Delta Z)}{\Delta Z} = \left[\frac{\delta\Omega}{\Omega} + \frac{\delta d}{d}\right] + \frac{2\bar{Z}}{\Omega d}\left[\delta\psi\Omega + \delta\Omega\psi\right] \tag{37}$$

which corresponds to eq.(9) of the manuscript.

Moreover, from eq.(28) and eq.(31) we have that $|Q| \equiv Z$, which means the distance, $\Delta R$, between the two targets, $Q_1$ and $Q_2$, is essentially equal to $\Delta Z$, hence the error on $\Delta R$, $\delta(\Delta R) \equiv \delta(\Delta Z)$ and the relative error on $\Delta R$ can be written as:

$$\frac{\delta(\Delta R)}{\Delta R} = \left[\frac{\delta\Omega}{\Omega} + \frac{\delta d}{d}\right] + \frac{2\bar{Z}}{\Omega d}\left[\delta\psi\Omega + \delta\Omega\psi\right] \tag{38}$$

## References

[1] W. Förstner and E. Gülch, "A fast operator for detection and precise location of distict point, corners and centres of circular features," in *Proceedings of the ISPRS Conference on Fast Processing of Photogrammetric Data*, Interlaken, 1987, pp. 281–305.
